# Supplementary material for: $O(a)$-improved QCD+QED Wilson Dirac operator on GPUs
Source: arXiv:2502.02490 source file (2025-02-04)
Supplement: Supplementary file 1 [file 99A-appendix.tex]

% This allows for compiling the file separately:
\documentclass[main.tex]{subfiles}

\begin{document}

todo

\end{document}
